# Supplementary material for: Instrumental Variables based DREM for Online Asymptotic Identification of Perturbed Linear Systems
Source: arXiv:2312.15631 ancillary file (2024-04-05)
Supplement: Supplementary file 1 [file supp.pdf]

# Supplement to “Instrumental Variables based DREM for Online Asymptotic Identification of Perturbed Linear Systems”

Anton Glushchenko, *Member, IEEE* and Konstantin Lastochkin

## Abstract

This article is a supplementary material for “Instrumental Variables based DREM for Online Asymptotic Identification of Perturbed Linear Systems” by the same authors. It provides some basic facts from the harmonic analysis, proof of one auxillary lemma and proofs of propositions 1, 2, 4-6 and theorem 1.

## APPENDIX A

This appendix contains some basic facts from the harmonic analysis [24, 25], and also includes the proof of one new lemma, which result is used in the proof of proposition 2.

**Definition A1.** A signal  $u(t) \in \mathbb{R}^n$  is said to be stationary if the following limit exists uniformly in  $t_0$ :

$$R_u(t) = \lim_{T \rightarrow \infty} \frac{1}{T} \int_{t_0}^{t_0+T} u(\tau) u^\top(t + \tau) d\tau, \quad (A1)$$

where  $R_u(t)$  stands for the autocovariance of  $u(t)$ .

**Definition A2.** A spectral measure of  $u(t) \in \mathbb{R}^n$  is the result of the Fourier transform of the autocovariance matrix  $R_u(t)$ :

$$S_u(\omega) = \int_{-\infty}^{+\infty} e^{-j\omega\tau} R_u(\tau) d\tau. \quad (A2)$$

**Proposition A1.** Let  $y(t) = H(s)u(t)$ , where  $H(s)$  is a proper stable  $m \times n$  matrix transfer function with real impulse response  $H(t)$ . Then, if  $u(t) \in \mathbb{R}^n$  is stationary, then the autocovariance and spectral measure between  $u(t)$  and  $y(t)$  are defined as follows:

$$R_{yu}(t) = \int_{-\infty}^{+\infty} \int_{-\infty}^{+\infty} H(\tau_1) R_u(t + \tau_1 - \tau_2) H^\top(\tau_2) d\tau_1 d\tau_2,$$

$$S_y(\omega) = H^*(j\omega) S_u(\omega) H^\top(j\omega) = H(-j\omega) S_u(\omega) H^\top(j\omega),$$

where  $H^*(j\omega)$  is a Hermitian matrix.

*Proof is given in [24, p. 42].*

**Definition A3.** A stationary signal  $u(t) \in \mathbb{R}^n$  is called sufficiently rich of order  $n$ , if the support of the spectral measure  $S_u(\omega)$  of  $u(t)$  contains at least  $n$  points.

**Definition A4.** A cross correlation between stationary signals  $u(t) \in \mathbb{R}^n$  and  $y(t) \in \mathbb{R}^m$  is defined to be the following limit, uniform in  $t_0$

$$R_{yu}(t) = \lim_{T \rightarrow \infty} \frac{1}{T} \int_{t_0}^{t_0+T} y(\tau) u^\top(t + \tau) d\tau, \quad (A3)$$

where  $R_{yu}(t)$  denotes the cross correlation between the signals  $u(t)$  and  $y(t)$ .

**Definition A5.** The cross spectral measure of the stationary signals  $u(t) \in \mathbb{R}^n$  and  $y(t) \in \mathbb{R}^m$  is called the Fourier transform of the cross correlation matrix:

$$S_{yu}(\omega) = \int_{-\infty}^{+\infty} e^{-j\omega\tau} R_{yu}(\tau) d\tau. \quad (A4)$$

**Proposition A2.** Let  $y(t) = H(s)u(t)$ , where  $H(s)$  is a proper stable  $m \times n$  matrix transfer function with impulse response  $H(t)$ . Then, if the signal  $u(t) \in \mathbb{R}^n$  is stationary, then the cross correlation and cross spectral measure of  $u(t)$  and  $y(t)$  are defined as follows:

$$R_{yu}(t) = \int_{-\infty}^{+\infty} H(\tau_1) R_u(t + \tau_1) d\tau_1,$$

$$S_{yu}(\omega) = H^*(j\omega) S_u(\omega),$$

where  $H^*(j\omega)$  is a Hermitian matrix.

*Proof is presented in [24, p. 44].*

**Lemma A1.** Let  $u(t) \in \mathbb{R}^n$  and  $y(t) \in \mathbb{R}^n$  be stationary signals. Then,  $\text{rank}\{R_{yu}(0)\} = n$  if and only if there exist  $T > 0$  and  $\alpha > 0$  such that

$$\left| \det \left\{ \int_t^{t+T} y(\tau) u^\top(\tau) d\tau \right\} \right| \geq \alpha > 0, \forall t \geq t_0. \quad (\text{A5})$$

*Proof of Lemma A1.*

**IF:** The definition of the cross correlation matrix implies that there exist  $T_0 > 0$  and scalars  $\ell_1, \ell_2$  of the same sign such that

$$\ell_1 R_{yu}(0) \leq \frac{1}{T_0} \int_{t_0}^{t_0+T_0} y(\tau) u^\top(\tau) d\tau \leq \ell_2 R_{yu}(0), \quad (\text{A6})$$

from which

$$\ell_1^n \det\{R_{yu}(0)\} \leq \frac{1}{T_0^n} \det \left\{ \int_{t_0}^{t_0+T_0} y(\tau) u^\top(\tau) d\tau \right\} \leq \ell_2^n \det\{R_{yu}(0)\},$$

and therefore, when  $\text{rank}\{R_{yu}(0)\} = n$ , then equation (A5) holds.

**IFF:** For all  $T > 0$  there exists a constant  $\alpha_0 > 0$  such that  $\alpha = \alpha_0 T^n > 0$ , which allows one to rewrite the inequality (A5) in the following form:

$$\left| \det \left\{ \int_t^{t+T} y(\tau) u^\top(\tau) d\tau \right\} \right| \geq \alpha_0 T^n > 0, \forall t \geq t_0. \quad (\text{A7})$$

The division of the left- and right-hand sides of equation (A7) by  $T^n$  yields:

$$\frac{1}{T^n} \left| \det \left\{ \int_t^{t+T} y(t) u^\top(t) d\tau \right\} \right| \geq \alpha_0 \quad (\text{A8})$$

and, consequently,

$$|\det\{R_{yu}(0)\}| = \lim_{T \rightarrow \infty} \frac{1}{T^n} \left| \det \left\{ \int_t^{t+T} y(t) u^\top(t) d\tau \right\} \right| \geq \lim_{T \rightarrow \infty} \alpha_0 = \alpha_0 > 0,$$

from which  $\text{rank}\{R_{yu}(0)\} = n$ .

## APPENDIX B

This appendix contains proofs of Theorem 1 and Propositions 1, 2, 4-6.

**Proof of Proposition 1.** As the polynomial  $\Lambda(s)$  is Hurwitz one, the disturbance  $w(t)$  is written as follows:

$$w(t) = \sum_{k=1}^{n_f} \delta_k \left[ \alpha_k^w \sin(\omega_k^f t) + \beta_k^w \cos(\omega_k^f t) \right] + \varepsilon_w(t), \quad (\text{B1})$$

where  $\varepsilon_w(t)$  stands for an exponentially vanishing disturbance, which is caused by the initial conditions and transients, and  $\alpha_k^w, \beta_k^w$  are some scalars.

The following scalar signal is introduced

$$\begin{aligned} \phi(t) &= [b_{n-1} \quad b_{n-2} \quad \dots \quad b_0] \varphi_y(t) = -[b_{n-1} \quad b_{n-2} \quad \dots \quad b_0] \frac{\lambda_{n-1}(s) Z(\theta, s)}{\Lambda(s) R(\theta, s)} [u(t) + f(t)] = \\ &= -[b_{n-1} \quad b_{n-2} \quad \dots \quad b_0] \frac{\lambda_{n-1}(s) Z(\theta, s)}{\Lambda(s) R(\theta, s)} u(t) - \frac{Z(\theta, s)}{R(\theta, s)} w(t), \end{aligned}$$

where  $\varphi_y(t) = [I_n \quad 0_{n \times n}] \varphi(t) = -\frac{\lambda_{n-1}(s)}{\Lambda(s)} y(t)$ .

As, according to assumption 1, the polynomial  $\Lambda(s) R(\theta, s)$  is Hurwitz one, then  $\phi(t)$  is written as:

$$\phi(t) = \sum_{k=1}^n \rho_k [\alpha_k^u \sin(\omega_k^u t) + \beta_k^u \cos(\omega_k^u t)] - \sum_{k=1}^{n_f} \delta_k [\alpha_k^{\bar{w}} \sin(\omega_k^f t) + \beta_k^{\bar{w}} \cos(\omega_k^f t)] + \varepsilon_{\bar{\varphi}}(t), \quad (\text{B2})$$

where  $\varepsilon_{\bar{\varphi}}(t)$  is an exponentially vanishing term, and  $\alpha_k^u, \beta_k^u, \alpha_k^{\bar{w}}, \beta_k^{\bar{w}}$  are some scalars.

As the signals (B2) and (B1) include terms with the same frequencies, then it can be concluded that:

$$\lim_{t \rightarrow \infty} \left| \int_{t_0}^t \phi(s) w(s) ds \right| = \infty, \quad (\text{B3})$$

which, as

$$\phi(t) = [b_{n-1} \quad b_{n-2} \quad \dots \quad b_0] [I_n \quad 0_{n \times n}] \varphi(t), \quad (\text{B4})$$

ensures existence of  $i \in \{1, \dots, 2n\}$  such that:  $\lim_{t \rightarrow \infty} \left| \int_{t_0}^t \varphi_i(s) w(s) ds \right| = \infty$ .

**Proof of Propostion 2.** Taking into account equations (1), (2), (12), the multiplication  $\zeta(t) \varphi^\top(t)$  is written as follows:

$$\begin{aligned} \zeta(t) \varphi^\top(t) &= \begin{bmatrix} -\frac{\lambda_{n-1}(s)}{\Lambda(s)} y_{iv}(t) \\ \frac{\lambda_{n-1}(s)}{\Lambda(s)} u(t) \end{bmatrix} \begin{bmatrix} -\frac{\lambda_{n-1}^\top(s)}{\Lambda(s)} y(t) & \frac{\lambda_{n-1}^\top(s)}{\Lambda(s)} u(t) \end{bmatrix} = \\ &= \begin{bmatrix} -\frac{\lambda_{n-1}(s)Z(\theta_{iv}, s)}{\Lambda(s)R(\theta_{iv}, s)} u(t) \\ \frac{\lambda_{n-1}(s)}{\Lambda(s)} u(t) \end{bmatrix} \begin{bmatrix} -\frac{\lambda_{n-1}^\top(s)Z(\theta, s)}{\Lambda(s)R(\theta, s)} u(t) & \frac{\lambda_{n-1}^\top(s)}{\Lambda(s)} u(t) \end{bmatrix} + \begin{bmatrix} -\frac{\lambda_{n-1}(s)Z(\theta_{iv}, s)}{\Lambda(s)R(\theta_{iv}, s)} u(t) \\ \frac{\lambda_{n-1}(s)}{\Lambda(s)} u(t) \end{bmatrix} \begin{bmatrix} -\frac{\lambda_{n-1}^\top(s)Z(\theta, s)}{\Lambda(s)R(\theta, s)} f(t) & 0 \end{bmatrix} = \\ &= \zeta(t) \bar{\varphi}^\top(t) + \zeta(t) \begin{bmatrix} -\frac{\lambda_{n-1}^\top(s)Z(\theta, s)}{\Lambda(s)R(\theta, s)} f(t) & 0 \end{bmatrix}, \end{aligned}$$

where

$$\begin{aligned} \zeta(t) &= \begin{bmatrix} -G(s) \frac{\lambda_{n-1}(s)Z(\theta, s)}{\Lambda(s)R(\theta, s)} u(t) \\ \frac{\lambda_{n-1}(s)}{\Lambda(s)} u(t) \end{bmatrix} = \begin{bmatrix} G(s) I_n & 0 \\ 0 & I_n \end{bmatrix} \bar{\varphi}(t), \\ \bar{\varphi}(t) &= \begin{bmatrix} -\frac{\lambda_{n-1}^\top(s)Z(\theta, s)}{\Lambda(s)R(\theta, s)} u(t) & \frac{\lambda_{n-1}^\top(s)}{\Lambda(s)} u(t) \end{bmatrix}^\top. \end{aligned}$$

**IF:** As  $\zeta(t)$  and  $\varphi(t)$  are stationary, then  $R_{\zeta\varphi}(0)$  is uniform with respect to  $t_0$ , which allows one to write:

$$\begin{aligned} R_{\zeta\varphi}(0) &= \lim_{T \rightarrow \infty} \frac{1}{T} \int_0^T \zeta(\tau) \varphi^\top(\tau) d\tau = \\ &= \lim_{T \rightarrow \infty} \frac{1}{T} \int_0^T \zeta(\tau) \bar{\varphi}^\top(\tau) d\tau + \lim_{T \rightarrow \infty} \frac{1}{T} \int_0^T \zeta(\tau) \begin{bmatrix} -\frac{\lambda_{n-1}^\top(s)Z(\theta, s)}{\Lambda(s)R(\theta, s)} f(\tau) & 0 \end{bmatrix} d\tau = \\ &= \frac{1}{2\pi} \int_{-\infty}^{+\infty} S_{\zeta\bar{\varphi}}(\omega) d\omega + \lim_{T \rightarrow \infty} \frac{1}{T} \int_0^T \zeta(\tau) \begin{bmatrix} -\frac{\lambda_{n-1}^\top(s)Z(\theta, s)}{\Lambda(s)R(\theta, s)} f(\tau) & 0 \end{bmatrix} d\tau, \end{aligned} \quad (\text{B5})$$

where  $S_{\zeta\bar{\varphi}}(\omega)$  stands for a cross spectral measure defined as (Proposition A2):

$$S_{\zeta\bar{\varphi}}(\omega) = M^*(j\omega) S_{\bar{\varphi}}(\omega), \quad (\text{B6})$$

where  $S_{\bar{\varphi}}(\omega)$  is a spectral measure of  $\bar{\varphi}(t)$ , which is defined as follows (Proposition A1):

$$S_{\bar{\varphi}}(\omega) = H(-j\omega) S_u(\omega) H^\top(j\omega). \quad (\text{B7})$$

As the signal  $u(t)$  has spectral lines at  $2n$  points, then the spectral measure  $S_u(\omega)$  is defined as follows:

$$S_u(\omega) = \sum_{i=1}^{2n} f_u(\omega_i) \delta(\omega - \omega_i), \quad (\text{B8})$$

where  $f_u(\omega_i) > 0$ .

Taking into consideration proof of Proposition 1, it follows that:

$$\lim_{T \rightarrow \infty} \frac{1}{T} \int_0^T \zeta(\tau) \begin{bmatrix} -\frac{\lambda_{n-1}^\top(s)Z(\theta, s)}{\Lambda(s)R(\theta, s)} f(\tau) & 0 \end{bmatrix} d\tau = 0. \quad (\text{B9})$$

Then, considering (B6)-(B8), it is obtained:

$$R_{\xi\bar{\varphi}}(0) = \frac{1}{2\pi} \sum_{i=1}^{2n} f_u(\omega_i) M^*(j\omega_i) H(-j\omega_i) H^\top(j\omega_i) = \frac{1}{2\pi} \mathcal{M} \mathcal{H}, \quad (\text{B10})$$

where

$$\begin{aligned} \mathcal{M} &= \begin{bmatrix} M^*(j\omega_1) & \dots & M^*(j\omega_{2n-1}) & M^*(j\omega_{2n}) \end{bmatrix}, \\ \mathcal{H} &= \begin{bmatrix} f_u(\omega_1) H(-j\omega_1) H^\top(j\omega_1) \\ \vdots \\ f_u(\omega_{2n-1}) H(-j\omega_{2n-1}) H^\top(j\omega_{2n-1}) \\ f_u(\omega_{2n}) H(-j\omega_{2n}) H^\top(j\omega_{2n}) \end{bmatrix}. \end{aligned}$$

According to the premises of proposition under consideration, it holds that

$$\mathcal{H} \in \mathbb{C}^{2n \times 2n}, \text{rank}\{\mathcal{H}\} = 2n, \text{rank}\{\mathcal{M}\} = 2n, \quad (\text{B11})$$

then

$$\text{rank}\{R_{\xi\bar{\varphi}}(0)\} = \text{rank}\{\mathcal{M}\} = 2n, \quad (\text{B12})$$

and, therefore, using Lemma A1, it is concluded that the condition (13) holds.

**IFF:** Let us assume that  $u(t)$  is sufficiently rich of order  $r < 2n$ , then  $R_{\xi\bar{\varphi}}(0)$  is written as:

$$R_{\xi\bar{\varphi}}(0) = \frac{1}{2\pi} \mathcal{M}_r \mathcal{H}_r, \quad (\text{B13})$$

where

$$\mathcal{M}_r = \begin{bmatrix} M^*(j\omega_1) & \cdots & M^*(j\omega_{r-1}) & M^*(j\omega_r) \end{bmatrix},$$

$$\mathcal{H}_r = \begin{bmatrix} f_u(\omega_1) H(-j\omega_1) H^\top(j\omega_1) \\ \vdots \\ f_u(\omega_{r-1}) H(-j\omega_{r-1}) H^\top(j\omega_{r-1}) \\ f_u(\omega_r) H(-j\omega_r) H^\top(j\omega_r) \end{bmatrix}.$$

So, the rank of  $R_{\xi\bar{\varphi}}(0)$  can be at most  $r < 2n$ , which contradicts the assumption that  $R_{\xi\bar{\varphi}}(0)$  is a full rank matrix.

**Proof of Propostion 4.** The solutions of the differential equations for  $\psi(t)$  and  $\vartheta(t)$  are written as:

$$\begin{aligned} \psi(t) &= \int_{\max(t_0, t-T)}^t \zeta(\tau) \varphi^\top(\tau) d\tau, \\ \vartheta(t) &= \int_{\max(t_0, t-T)}^t \zeta(\tau) z(\tau) d\tau = \\ &= \int_{\max(t_0, t-T)}^t \zeta(\tau) \varphi^\top(\tau) d\tau \theta + \int_{\max(t_0, t-T)}^t \zeta(\tau) w(\tau) d\tau = \psi(t) \theta + \varepsilon(t). \end{aligned} \quad (\text{B14})$$

To complete the proof, the following functions are introduced:

$$\begin{aligned} K_1(t) &= F(t) Y(t), \\ K_2(t) &= F(t) \Phi(t), \\ K_3(t) &= F(t) W(t) \end{aligned} \quad (\text{B15})$$

and their derivatives are written:

$$\begin{aligned} \dot{K}_1(t) &= \dot{F}(t) Y(t) + F(t) \dot{Y}(t) = \left( \dot{F}(t) - \dot{F}(t) \right) Y(t) + \dot{F}(t) \vartheta(t) = \dot{F}(t) \vartheta(t), \\ \dot{K}_2(t) &= \dot{F}(t) \psi(t), \\ \dot{K}_3(t) &= \dot{F}(t) \varepsilon(t), \end{aligned} \quad (\text{B16})$$

which allows one to obtain:

$$Y(t) = \frac{1}{F(t)} \int_{t_0}^t \dot{F}(s) \vartheta(s) ds = \frac{1}{F(t)} \int_{t_0}^t \dot{F}(s) \psi(s) \theta ds + \frac{1}{F(t)} \int_{t_0}^t \dot{F}(s) \varepsilon(s) ds = \Phi(t) \theta + W(t). \quad (\text{B17})$$

**Proof of Propostion 5. 1)** Using (B14)-(B17), the solution of the differential equation for  $\Phi(t)$  is obtained in the following form:

$$\Phi(t) = \frac{1}{F(t)} \int_{t_0}^t \dot{F}(s) \int_{\max(t_0, s-T)}^s \zeta(\tau) \varphi^\top(\tau) d\tau ds. \quad (\text{B18})$$

Owing to the fact that the condition (13) holds, there exist matrices  $R_-$  and  $R_+$  such that:

$$\begin{aligned} \int_{\frac{t}{t+T}}^{\frac{t+T}{t}} \zeta(\tau) \varphi^\top(\tau) d\tau &\leq R_-, \\ \int_{\frac{t}{t+T}}^{\frac{t+T}{t}} \zeta(\tau) \varphi^\top(\tau) d\tau &\geq R_+, \end{aligned} \quad (\text{B19})$$

where  $\det \{R_-\} = -\alpha$ ,  $\det \{R_+\} = \alpha$ .

Then for all  $t \geq t_0 + T$  the following bounds also exist:

$$\begin{aligned} \int_{\max(t_0, t-T)}^t \zeta(\tau) \varphi^\top(\tau) d\tau &\leq R_-, \\ \int_{\max(t_0, t-T)}^t \zeta(\tau) \varphi^\top(\tau) d\tau &\geq R_+, \end{aligned}$$

from which it is obtained that:

$$\begin{aligned} \Phi(t) &= \frac{1}{F(t)} \int_{t_0}^{t_0+T} \dot{F}(s) \int_{\max(t_0, s-T)}^s \zeta(\tau) \varphi^\top(\tau) d\tau ds + \frac{1}{F(t)} \int_{t_0+T}^t \dot{F}(s) \int_{\max(t_0, s-T)}^s \zeta(\tau) \varphi^\top(\tau) d\tau ds \geq \\ &\geq \frac{1}{F(t)} \int_{t_0}^{t_0+T} \dot{F}(s) \int_{\max(t_0, s-T)}^s \zeta(\tau) \varphi^\top(\tau) d\tau ds + \frac{1}{F(t)} \int_{t_0+T}^t \dot{F}(s) ds R_+ = \\ &= \frac{1}{F(t)} \int_{t_0}^{t_0+T} \dot{F}(s) \int_{\max(t_0, s-T)}^s \zeta(\tau) \varphi^\top(\tau) d\tau ds + \frac{F(t)-F(t_0+T)}{F(t)} R_+ \geq \\ &\geq \frac{1}{F(t)} \int_{t_0}^{t_0+T} \dot{F}(s) \int_{\max(t_0, s-T)}^s \zeta(\tau) \varphi^\top(\tau) d\tau ds + c R_+, \end{aligned} \quad (\text{B20})$$

$$\begin{aligned}
\Phi(t) &= \frac{1}{F(t)} \int_{t_0}^{t_0+T} \dot{F}(s) \int_{\max(t_0, s-T)}^s \zeta(\tau) \varphi^\top(\tau) d\tau ds + \\
&+ \frac{1}{F(t)} \int_{t_0+T}^t \dot{F}(s) \int_{\max(t_0, s-T)}^s \zeta(\tau) \varphi^\top(\tau) d\tau ds \leq \frac{1}{F(t)} \int_{t_0}^{t_0+T} \dot{F}(s) \int_{\max(t_0, s-T)}^s \zeta(\tau) \varphi^\top(\tau) d\tau ds + \frac{1}{F(t)} \int_T^t \dot{F}(s) ds R_- = \\
&= \frac{1}{F(t)} \int_{t_0}^{t_0+T} \dot{F}(s) \int_{\max(t_0, s-T)}^s \zeta(\tau) \varphi^\top(\tau) d\tau ds + \frac{F(t)-F(T)}{F(t)} R_- \leq \\
&\leq \frac{1}{F(t)} \int_{t_0}^{t_0+T} \dot{F}(s) \int_{\max(t_0, s-T)}^s \zeta(\tau) \varphi^\top(\tau) d\tau ds + cR_-,
\end{aligned}$$

where  $c > 0$  is an arbitrary scalar.

Then, as  $F(t)$  is the increasing function, the first summands of the above-given bounds are vanishing, and there exist a time instant  $T_\Delta \geq t_0 + T$  and a scalar  $\Delta_{LB} > 0$  such that  $|\Delta(t)| \geq \Delta_{LB} > 0$  for all  $t \geq T_\Delta$ .

2) As according to assumption 1 the signals  $y(t)$ ,  $u(t)$ ,  $f(t)$  are bounded, then, owing to the fact that  $\Lambda(s)$  is a Hurwitz polynomial, the signals  $\zeta(t)$ ,  $\varphi(t)$  are also bounded.

From which, as  $\dot{F}(t)$  is monotonically increasing, we have:

$$\|\Phi(t)\| \leq \left\| \frac{1}{F(t)} \int_{t_0}^t \dot{F}(s) \int_{\max(t_0, s-T)}^s \zeta(\tau) \varphi^\top(\tau) d\tau ds \right\| \leq T \frac{F(t)-F(t_0)}{F(t)} \sup_t \|\zeta(t) \varphi^\top(t)\|, \quad (\text{B21})$$

and, therefore, owing to the definition

$$\Delta(t) := \det \{\Phi(t)\},$$

there exists a scalar  $\Delta_{UB} > 0$  such that  $|\Delta(t)| \leq \Delta_{UB}$ .

3) According to Holder inequality, for any  $1 \leq a, b \leq \infty$  such that  $\frac{1}{a} + \frac{1}{b} = 1$  we have:

$$|W_i(t)| = \frac{1}{F(t)} \left| \int_{t_0}^t \dot{F}(\tau) \int_{\max(t_0, \tau-T)}^\tau \zeta_i(s) w(s) ds d\tau \right| \leq \frac{1}{F(t)} \sqrt[a]{\int_{t_0}^t \dot{F}^a(\tau) d\tau} \sqrt[b]{\int_{\max(t_0, t-T)}^t (\zeta_i(\tau) w(\tau))^b d\tau}. \quad (\text{B22})$$

The second multiplier of the upper bound from (B22) for any  $1 \leq a \leq \infty$  satisfies the inequality:

$$\sqrt[a]{\int_{t_0}^t \dot{F}^a(\tau) d\tau} = p \sqrt[a]{\int_{t_0}^t \tau^{a(p-1)} d\tau} = \frac{p}{\sqrt[a]{a(p-1)+1}} \sqrt[a]{t^{a(p-1)+1} - t_0^{a(p-1)+1}} \leq \frac{p}{\sqrt[a]{a(p-1)+1}} t^{p-1} \sqrt[a]{t} = \frac{1}{\sqrt[a]{a(p-1)+1}} \dot{F}(t) \sqrt[a]{t}.$$

Now we choose  $b = 1$ , and, consequently, the following inequality is obtained for any  $t \geq t_0$ :

$$\sqrt[a]{\int_{t_0}^t \dot{F}^a(\tau) d\tau} \leq \frac{1}{\sqrt[a]{a(p-1)+1}} \dot{F}(t) \sqrt[a]{t} = \dot{F}(t),$$

that involves the following upper bound for  $W_i(t)$ :

$$|W_i(t)| \leq \frac{\dot{F}(t)}{F(t)} \int_{\max(t_0, t-T)}^t \zeta_i(\tau) w(\tau) d\tau \leq \frac{\dot{F}(t)}{F(t)} c_W,$$

where  $c_W := T \max_i \sup_t \left| \int_{t_0}^t \zeta_i(s) w(s) ds \right| < \infty$  exists as condition (9) is met.

As the regressor  $\Phi(t)$  is bounded (B21), then the matrix  $\text{adj} \{\Phi(t)\}$  is also bounded, and therefore there exists a scalar  $c_W > 0$  such that the inequality (18) holds.

According to the bound (18) and taking into account inequality  $F_0 > t_0^p$ , the following upper bound exists for any  $l \in (1, \infty)$ :

$$\sqrt[l]{\int_{t_0}^t \mathcal{W}_i^l(\tau) d\tau} \leq c_W \sqrt[l]{\int_{t_0}^t \left( \frac{\dot{F}(\tau)}{F(\tau)} \right)^l d\tau} = c_W p \sqrt[l]{\int_{t_0}^t \left( \frac{\tau^{p-1}}{\tau^p - t_0^p + F_0} \right)^l d\tau} = c_W p \sqrt[l]{\int_{t_0}^t \left( \frac{1}{\tau + \frac{F_0 - t_0^p}{\tau^{p-1}}} \right)^l d\tau} < c_W p \sqrt[l]{\int_{t_0}^t \left( \frac{1}{\tau} \right)^l d\tau} = \infty,$$

and, consequently,  $\mathcal{W}_i \in L_l$ , which completes the proof.

**Proof of Theorem 1.** The following signal is introduced:

$$\kappa(t) = (t + F_0) \tilde{\theta}_i(t) \quad (\text{B23})$$

and its derivative is written with respect to (17):

$$\begin{aligned}
\dot{\kappa}(t) &= \tilde{\theta}_i(t) - \gamma \Delta^2(t) (t + F_0) \tilde{\theta}_i(t) + \gamma \Delta(t) (t + F_0) \mathcal{W}_i(t) = \\
&= -\gamma \Delta^2(t) \kappa(t) + \gamma \Delta(t) (t + F_0) \mathcal{W}_i(t) + \tilde{\theta}_i(t).
\end{aligned} \quad (\text{B24})$$

Following (B23), it can be concluded from the boundedness of  $\kappa(t)$  and  $\tilde{\theta}_i(t)$  that  $\tilde{\theta}_i(t)$  converges to zero. Therefore, to prove the theorem, the boundedness of  $\tilde{\theta}_i(t)$  and  $\kappa(t)$  are investigated.

To obtain the bound of  $\tilde{\theta}_i(t)$ , the differential equation (17) is solved:

$$\tilde{\theta}_i(t) = \phi(t, t_0) \tilde{\theta}_i(t_0) + \gamma \int_{t_0}^t \phi(t, s) \Delta(s) \mathcal{W}_i(s) ds, \quad (\text{B25})$$

where

$$\phi(t, \tau) = \exp \left( -\gamma \int_{\tau}^t \Delta^2(s) ds \right). \quad (\text{B26})$$

Further, for all  $t \geq t_0$  it is written:

$$\begin{aligned} \left| \tilde{\theta}_i(t) \right| &\leq \phi(t, t_0) \left| \tilde{\theta}_i(t_0) \right| + \gamma \int_{t_0}^t |\phi(t, s) \Delta(s)| |\mathcal{W}_i(s)| ds \leq \\ &\leq \phi(t, t_0) \left| \tilde{\theta}_i(t_0) \right| + \gamma \sqrt{\int_{t_0}^t \phi^2(t, s) \Delta^2(s) ds \int_{t_0}^t \mathcal{W}_i^2(s) ds}, \end{aligned} \quad (\text{B27})$$

where the Cauchy–Schwarz inequality is used in the last step.

The equality

$$\frac{\partial}{\partial s} \phi^2(t, s) = 2\gamma \phi^2(t, s) \Delta^2(s)$$

allows one to rewrite equation (B27) as follows:

$$\left| \tilde{\theta}_i(t) \right| \leq \phi(t, t_0) \left| \tilde{\theta}_i(t_0) \right| + \sqrt{\frac{\gamma}{2}} \sqrt{1 - \phi^2(t, t_0)} \sqrt{\int_{t_0}^t \mathcal{W}_i^2(s) ds}. \quad (\text{B28})$$

As it holds that:

$$\begin{aligned} \phi(t, t_0) &\leq 1, \quad \sqrt{1 - \phi^2(t, t_0)} \leq 1, \\ \sqrt{\int_{t_0}^t \mathcal{W}_i^2(s) ds} &\leq c_{\mathcal{W}} \sqrt{\int_{t_0}^t \frac{\dot{F}^2(s)}{F^2(s)} ds} < \infty, \end{aligned} \quad (\text{B29})$$

then, owing to (B28), there exists  $\tilde{\theta}_{\max} > 0$  such that  $\left| \tilde{\theta}_i(t) \right| \leq \tilde{\theta}_{\max}$  for all  $t \geq t_0$ .

Taking into account the obtained bounds, the boundedness of the variable  $\kappa(t)$  is to be proved. For this purpose, a quadratic form is introduced:

$$V = \frac{1}{2} \kappa^2. \quad (\text{B30})$$

The derivative of (B30) with respect to (B24) is:

$$\dot{V} = -\gamma \Delta^2 \kappa^2 + \gamma \Delta \kappa (t + F_0) \mathcal{W}_i + \kappa \tilde{\theta}_i. \quad (\text{B31})$$

Using the inequalities:

$$\begin{aligned} (t + F_0) \Delta \kappa \mathcal{W}_i &\leq \delta^{-1} \Delta^2 \kappa^2 + \delta (t + F_0)^2 \mathcal{W}_i^2, \quad \delta > 0, \\ (t + F_0)^2 \mathcal{W}_i^2(t) &\leq \frac{(t + F_0)^2 \dot{F}^2 c_{\mathcal{W}}^2}{F^2} = \frac{(t + F_0)^2 p^2 t^{2p-2} c_{\mathcal{W}}^2}{(t^p + F_0)^2} \leq \mathcal{W}_{\text{UB}}^2 < \infty, \\ \kappa \tilde{\theta}_i &\leq \rho^{-1} \kappa^2 + \rho \tilde{\theta}_i^2, \quad \rho > 0, \end{aligned} \quad (\text{B32})$$

it is written that:

$$\dot{V} \leq -2\gamma \left( (1 - \delta^{-1}) \Delta^2 - \rho^{-1} \gamma^{-1} \right) V + \delta \mathcal{W}_{\text{UB}}^2 + \rho \tilde{\theta}_i^2. \quad (\text{B33})$$

According to the premises of theorem, for all  $t \geq T_{\Delta}$  it holds that  $|\Delta(t)| \geq \Delta_{\text{LB}} > 0$ , and therefore, there exist constants  $\delta > 0$ ,  $\rho > 0$  and  $\eta_{\min} > 0$  such that

$$\gamma \left( (1 - \delta^{-1}) \Delta^2 - \rho^{-1} \gamma^{-1} \right) \geq \eta_{\min} > 0. \quad (\text{B34})$$

Considering (B34), the solution of equation (B33) is obtained as:

$$V(t) \leq e^{-2\eta_{\min}(t-T_{\Delta})} V(T_{\Delta}) + \frac{1}{2\eta_{\min}} \left[ \delta \mathcal{W}_{\text{UB}}^2 + \rho \tilde{\theta}_{\max}^2 \right], \quad (\text{B35})$$

from which it follows that there exists a scalar  $\kappa_{\max}$  such that  $|\kappa(t)| \leq \kappa_{\max}$  for all  $t \geq T_{\Delta}$ .

As  $t + F_0 \rightarrow \infty$  when  $t \rightarrow \infty$ , and  $|\kappa(t)| \leq \kappa_{\max}$ , then from (B23) it follows that (3) holds.

If condition (19) is met, then  $\mathcal{W}_i(t) = 0$  for all  $t \geq T$ , and from equation (B25) it is obvious that

$$\forall t \geq T_{\Delta} \quad \left| \tilde{\theta}_i(t) \right| \leq e^{-\gamma \Delta_{\text{LB}}(t-T_{\Delta})} \left| \tilde{\theta}_i(T_{\Delta}) \right| \quad \forall i = 1, \dots, 2n,$$

which completes the proof.

**Proof of Propostion 6.** Equation (20) is substituted into (1) and vice versa to obtain:

$$\begin{aligned} u(t) &= W_{cl}(\theta, s) R(\theta, s) \left[ r(t) + \frac{P_y(\kappa, s) Z(\theta, s) Q_r(\kappa, s)}{Q_y(\kappa, s) R(\theta, s) P_r(\kappa, s)} f(t) \right], \\ y(t) &= W_{cl}(\theta, s) Z(\theta, s) \left[ r(t) + \frac{Q_r(\kappa, s)}{P_r(\kappa, s)} f(t) \right]. \end{aligned} \quad (\text{B36})$$

Considering (2), (21) and (B36), the multiplication  $\zeta(t) \varphi^\top(t)$  is rewritten as:

$$\begin{aligned}
\zeta(t) \varphi^\top(t) &= \begin{bmatrix} -\frac{\lambda_{n-1}(s)}{\Lambda(s)} y_{iv}(t) \\ \frac{\lambda_{n-1}(s)}{\Lambda(s)} u(t) \end{bmatrix} \begin{bmatrix} -\frac{\lambda_{n-1}^\top(s)}{\Lambda(s)} y(t) & \frac{\lambda_{n-1}^\top(s)}{\Lambda(s)} u(t) \end{bmatrix} = \\
&= \begin{bmatrix} -\frac{\lambda_{n-1}(s) W_{cl}(\theta_{iv}, s) Z(\theta_{iv}, s)}{\Lambda(s)} r(t) \\ \frac{\lambda_{n-1}(s) W_{cl}(\theta_{iv}, s) R(\theta_{iv}, s)}{\Lambda(s)} r(t) \end{bmatrix} \begin{bmatrix} -\frac{\lambda_{n-1}(s) W_{cl}(\theta, s) Z(\theta, s)}{\Lambda(s)} \left[ r(t) + \frac{Q_r(\kappa, s)}{P_r(\kappa, s)} f(t) \right] \\ \frac{\lambda_{n-1}(s) W_{cl}(\theta, s) R(\theta, s)}{\Lambda(s)} \left[ r(t) + \frac{P_y(\kappa, s) Z(\theta, s) Q_r(\kappa, s)}{Q_y(\kappa, s) R(\theta, s) P_r(\kappa, s)} f(t) \right] \end{bmatrix}^\top = \\
&= \begin{bmatrix} -\frac{\lambda_{n-1}(s) W_{cl}(\theta_{iv}, s) Z(\theta_{iv}, s)}{\Lambda(s)} r(t) \\ \frac{\lambda_{n-1}(s) W_{cl}(\theta_{iv}, s) R(\theta_{iv}, s)}{\Lambda(s)} r(t) \end{bmatrix} \begin{bmatrix} -\frac{\lambda_{n-1}^\top(s) W_{cl}(\theta, s) Z(\theta, s)}{\Lambda(s)} r(t) & \frac{\lambda_{n-1}^\top(s) W_{cl}(\theta, s) R(\theta, s)}{\Lambda(s)} r(t) \end{bmatrix} + \\
&+ \begin{bmatrix} -\frac{\lambda_{n-1}(s) W_{cl}(\theta_{iv}, s) Z(\theta_{iv}, s)}{\Lambda(s)} r(t) \\ \frac{\lambda_{n-1}(s) W_{cl}(\theta_{iv}, s) R(\theta_{iv}, s)}{\Lambda(s)} r(t) \end{bmatrix} \times \begin{bmatrix} -\frac{\lambda_{n-1}(s) W_{cl}(\theta, s) Z(\theta, s) Q_r(\kappa, s)}{\Lambda(s) P_r(\kappa, s)} f(t) \\ \frac{\lambda_{n-1}(s) W_{cl}(\theta, s) R(\theta, s) P_y(\kappa, s) Z(\theta, s) Q_r(\kappa, s)}{\Lambda(s) Q_y(\kappa, s) R(\theta, s) P_r(\kappa, s)} f(t) \end{bmatrix}^\top = \\
&= \zeta(t) \bar{\varphi}^\top(t) + \zeta(t) d(t),
\end{aligned} \tag{B37}$$

where

$$\begin{aligned}
\zeta(t) &= \begin{bmatrix} -G_1(s) \frac{\lambda_{n-1}(s) W_{cl}(\theta, s) Z(\theta, s)}{\Lambda(s)} r(t) \\ G_2(s) \frac{\lambda_{n-1}(s) W_{cl}(\theta, s) R(\theta, s)}{\Lambda(s)} r(t) \end{bmatrix} = \begin{bmatrix} G_1(s) I_n & 0 \\ 0 & G_2(s) I_n \end{bmatrix} \bar{\varphi}(t), \\
\bar{\varphi}(t) &= \begin{bmatrix} -\frac{\lambda_{n-1}(s) W_{cl}(\theta, s) Z(\theta, s)}{\Lambda(s)} r(t) \\ \frac{\lambda_{n-1}(s) W_{cl}(\theta, s) R(\theta, s)}{\Lambda(s)} r(t) \end{bmatrix}, \\
d(t) &= \begin{bmatrix} -\frac{\lambda_{n-1}(s) W_{cl}(\theta, s) Z(\theta, s) Q_r(\kappa, s)}{\Lambda(s) P_r(\kappa, s)} f(t) \\ \frac{\lambda_{n-1}(s) W_{cl}(\theta, s) R(\theta, s) P_y(\kappa, s) Z(\theta, s) Q_r(\kappa, s)}{\Lambda(s) Q_y(\kappa, s) R(\theta, s) P_r(\kappa, s)} f(t) \end{bmatrix}.
\end{aligned} \tag{B38}$$

Further proof is done by analogy with the one of proposition 2.
